# Supplementary material for: On the well-posedness of uncalibrated photometric stereo under general lighting
Source: arXiv:1911.07268 source file (2020-09-17)
Supplement: Supplementary file 1 [file 09appendix.tex]

\section*{Appendix 3: Perspective integrability constraint, and Corollary \ref{cor:2}}
%\label{sec:app3}

The proof of Theorem \ref{thm:3} uses the expression of the integrability constraint under perspective projection. This expression is given by Corollary \ref{cor:2}, which we prove in this section.

Let $z:\,\Omega \to \R$ a twice differentiable depth map of an object, $\mathbf{n} := \left[n_1,n_2,n_3\right]^\top:\,\Omega \to \mathbb{S}^2 \subset \R^3$ its normal field, and let us define the $\log$ depth map as: 
\begin{align}
    & \tilde{z} = \text{log}(z),
\end{align}
and denote:
\begin{align}
    & p = -\dfrac{n_1}{n_3}, \qquad q = -\dfrac{n_2}{n_3}.
\end{align}

\begin{proposition}
\label{prop:9}
The gradient of the $\log$-depth map $\tilde{z} = \log z$ is given by: 
\begin{align}
    & \nabla \tilde{z} = \left[\hat{p},\hat{q}\right]^\top,\text{~with} \\
    & \hat{p} = \dfrac{p}{f - up - vq} \text{~~and~~} \hat{q} = \dfrac{q}{f - up - vq}. 
\end{align}
\end{proposition}
\begin{proof}
By definition of $\hat{p}$ and using the relationship~\eqref{eq:normal_perspective} between the normal and depth maps:
\begin{equation}
    \hat{p} = \dfrac{p}{f - up - vq} = \dfrac{-n_1}{f n_3 + u n_1 + v n_2} = \dfrac{z_u}{z} = \tilde{z}_{u}. 
\end{equation}
Similarly, we show that $\hat{q} = \tilde{z}_{v}$.
\end{proof}

\begin{proposition}
\label{prop:8}
Integrability of the depth map and integrability of the $\log$-depth map are equivalent, i.e.:
\begin{equation}
    z_{uv} = z_{vu} \iff \tilde{z}_{uv} = \tilde{z}_{vu}.
\end{equation}
\end{proposition}
\begin{proof}
Assuming $z >0$:
\begin{align}
    z_{uv} = z_{vu} & \iff \dfrac{z_{uv}z - z_u z_v}{z^2} = \dfrac{z_{vu}z - z_u z_v}{z^2}, \\
    & \iff \left(\dfrac{z_u}{z}\right)_v = \left(\dfrac{z_v}{z}\right)_u, \\
    & \iff \tilde{z}_{uv} = \tilde{z}_{vu}.
\end{align}
\end{proof}

\begin{corollary}
\label{cor:2}
Let $\mathbf{m} = \left[c_1,c_2,c_3,c_4\right]^\top:\,\Omega \to \R^4$ a field with the form of Equation~\eqref{eq:16}. The underlying normal field is integrable iff the following relationship holds over~$\Omega$:
\begin{equation}
   u(c_{2}c_{3u} - c_{2u}c_{3}) + v(c_{2}c_{3v} - c_{2v}c_{3}) + f(c_{2}c_{4v} - c_{2v}c_{4}) + f(c_{3u}c_{4} - c_{3}c_{4u}) = 0. 
\end{equation}
\end{corollary}

\newpage
